# Supplementary material for: Active Inference for Physical AI Agents -- An Engineering Perspective
Source: arXiv:2603.20927 source file (2026-03-21)
Supplement: Supplementary file 1 [file appendix-football-example.tex]

\section{Concrete Football Play Walkthrough}\label{app:football-play}

This appendix provides a small quantitative example of active inference
applied to the football scenario of
Section~\ref{sec:aif-robot-football}. The goal is not realism but to
show explicitly how a ``reposition $\rightarrow$ pass'' behavior arises
from EFE minimization in a simple probabilistic model.

\subsection{Scenario}\label{app:football-scenario}

Player $P_1$ has the ball and considers passing to teammate $P_2$. The
passing lane may be open or blocked by an opponent, but $P_1$'s current
view is partially occluded. Two options are available:
\begin{itemize}
    \item \emph{Pass immediately:} commit to the pass without further
    information.
    \item \emph{Reposition first:} move to a better vantage point,
    observe the lane more clearly, and then either pass to $P_2$ (if
    the lane appears clear) or recycle the ball safely to $P_3$ (if the
    lane appears blocked).
\end{itemize}
We model this as a two-step decision and show that EFE minimization
selects the reposition-then-pass sequence.

\subsection{Variables and Domains}\label{app:football-variables}

\begin{itemize}
    \item \textbf{Lane state} $x \in \{O, B\}$: the passing lane is
    open ($O$) or blocked ($B$).
    \item \textbf{Lane observation} $y \in \{c, u\}$: the lane appears
    clear ($c$) or unclear ($u$).
    \item \textbf{Outcome state} $x' \in \{A, T\}$: the play results
    in attacking progress ($A$) or turnover ($T$).
    \item \textbf{Action} $u \in \{u_{\mathrm{pass}},
    u_{\mathrm{rep}}, u_{\mathrm{rec}}\}$: pass to $P_2$, reposition,
    or recycle to $P_3$.
\end{itemize}

\subsection{Model Assumptions}\label{app:football-model}

All probabilistic assumptions are collected here; no additional model
specifications appear in later subsections.

\subsubsection*{Prior}\label{app:prior}

The agent's initial belief reflects slight confidence that the lane is
open, with substantial residual uncertainty:
\begin{equation}\label{eq:app-prior}
    p(x{=}O) = 0.6\,,\quad p(x{=}B) = 0.4\,.
\end{equation}

\subsubsection*{Lane observation model}\label{app:obs-model}

When passing immediately, the observation is weakly informative (the
current vantage point is poor):
\begin{equation}\label{eq:app-obs-pass}
    p(y{=}c \,|\, x{=}O,\, u_{\mathrm{pass}}) = 0.6\,,\qquad
    p(y{=}c \,|\, x{=}B,\, u_{\mathrm{pass}}) = 0.4\,.
\end{equation}
After repositioning, the observation is much sharper:
\begin{equation}\label{eq:app-obs-rep}
    p(y{=}c \,|\, x{=}O,\, u_{\mathrm{rep}}) = 0.9\,,\qquad
    p(y{=}c \,|\, x{=}B,\, u_{\mathrm{rep}}) = 0.2\,.
\end{equation}

\subsubsection*{Transition model}\label{app:transition-model}

Passing through an open lane is likely to create attacking progress;
passing through a blocked lane is likely to result in turnover:
\begin{equation}\label{eq:app-trans-pass}
    p(x'{=}A \,|\, x{=}O,\, u_{\mathrm{pass}}) = 0.9\,,\qquad
    p(x'{=}A \,|\, x{=}B,\, u_{\mathrm{pass}}) = 0.2\,.
\end{equation}
Recycling safely to $P_3$ yields a moderate chance of continued
attacking play, regardless of the lane state:
\begin{equation}\label{eq:app-trans-rec}
    p(x'{=}A \,|\, u_{\mathrm{rec}}) = 0.5\,.
\end{equation}

\subsubsection*{Preference model}\label{app:preference-model}

The player strongly prefers attacking progress over turnover:
\begin{equation}\label{eq:app-pref}
    \hat{p}(x'{=}A) = 0.9\,,\qquad \hat{p}(x'{=}T) = 0.1\,.
\end{equation}

\subsubsection*{Policy prior}\label{app:policy-prior}

We assume a uniform prior over policies, so the empirical prior $P(u)$
and complexity $C(u)$ terms in \eqref{eq:GuCuPu-def} do not affect
policy ranking. Policy selection is therefore governed entirely by the
EFE $G(u)$.

\subsection{First-Step Policy Selection}\label{app:step1}

The agent selects $u_1$ by comparing the EFE
\eqref{eq:Gu-def} for each first-step policy:
\begin{equation}\label{eq:app-efe}
    G(u_1) =
    \underbrace{\mathrm{KL}\!\big(q(x' | u_1)\,\big\|\,\hat{p}(x')\big)}_{\text{risk}}
    +
    \underbrace{\mathbb{E}_{q(x | u_1)}\!\big[\mathbb{H}[y \,|\, x]\big]}_{\text{ambiguity}}\,,
\end{equation}
where $q(x | u_1) = p(x)$ (the prior does not depend on $u_1$) and we write
$h(p) \triangleq -p\log p - (1{-}p)\log(1{-}p)$ for the binary
entropy in nats.

\subsubsection*{Immediate passing}\label{app:efe-pass}

The predicted outcome distribution under immediate passing is
\begin{equation}
    q(x'{=}A \,|\, u_{\mathrm{pass}})
    = 0.6 \cdot 0.9 + 0.4 \cdot 0.2
    = 0.62\,.
\end{equation}
The risk measures how far this prediction lies from the preferred
outcome:
\begin{equation}
    \mathrm{KL}\!\big(q(x'|u_{\mathrm{pass}})\,\big\|\,\hat{p}(x')\big)
    = 0.62\ln\!\tfrac{0.62}{0.9} + 0.38\ln\!\tfrac{0.38}{0.1}
    \approx 0.276\,.
\end{equation}
The ambiguity measures how uninformative the lane observation would be.
Since the observation likelihoods under passing are nearly symmetric
\eqref{eq:app-obs-pass}, the observation resolves little uncertainty:
\begin{equation}
    \mathbb{E}_{p(x)}\!\big[\mathbb{H}[y | x]\big]
    = 0.6 \cdot h(0.6) + 0.4 \cdot h(0.4)
    = h(0.6)
    \approx 0.673\,.
\end{equation}
Therefore
\begin{equation}\label{eq:app-G-pass}
    G(u_{\mathrm{pass}}) \approx 0.276 + 0.673 = 0.949\,.
\end{equation}

\subsubsection*{Repositioning}\label{app:efe-rep}

Under $u_{\mathrm{rep}}$, the agent plans to observe $y$ and then act
contingently: pass if $y{=}c$, recycle if $y{=}u$. This contingent
strategy yields an effective transition that marginalizes over the
observation:
\begin{equation}
    p(x'{=}A | x,\, u_{\mathrm{rep}})
    = p(y{=}c | x,\, u_{\mathrm{rep}})\,p(x'{=}A | x,\, u_{\mathrm{pass}})
    + p(y{=}u | x,\, u_{\mathrm{rep}})\,p(x'{=}A | u_{\mathrm{rec}})\,.
\end{equation}
Evaluating for each lane state:
\begin{align}
    p(x'{=}A \,|\, x{=}O,\, u_{\mathrm{rep}})
    &= 0.9 \cdot 0.9 + 0.1 \cdot 0.5 = 0.86\,,\notag\\
    p(x'{=}A \,|\, x{=}B,\, u_{\mathrm{rep}})
    &= 0.2 \cdot 0.2 + 0.8 \cdot 0.5 = 0.44\,.
\end{align}
The predicted outcome distribution is therefore
\begin{equation}
    q(x'{=}A \,|\, u_{\mathrm{rep}})
    = 0.6 \cdot 0.86 + 0.4 \cdot 0.44
    = 0.692\,.
\end{equation}
The risk is
\begin{equation}
    \mathrm{KL}\!\big(q(x'|u_{\mathrm{rep}})\,\big\|\,\hat{p}(x')\big)
    = 0.692\ln\!\tfrac{0.692}{0.9} + 0.308\ln\!\tfrac{0.308}{0.1}
    \approx 0.165\,.
\end{equation}
The sharper observation model \eqref{eq:app-obs-rep} yields lower
ambiguity:
\begin{equation}
    \mathbb{E}_{p(x)}\!\big[\mathbb{H}[y | x]\big]
    = 0.6 \cdot h(0.9) + 0.4 \cdot h(0.2)
    \approx 0.195 + 0.200
    = 0.395\,.
\end{equation}
Therefore
\begin{equation}\label{eq:app-G-rep}
    G(u_{\mathrm{rep}}) \approx 0.165 + 0.395 = 0.560\,.
\end{equation}

\subsubsection*{Action selection}\label{app:step1-select}

Comparing the two policies:
\begin{equation}
    G(u_{\mathrm{rep}}) = 0.560 \;<\; G(u_{\mathrm{pass}}) = 0.949\,,
\end{equation}
so the agent selects $u_1 = u_{\mathrm{rep}}$: reposition before
committing. Both terms favor repositioning: the risk is lower
(the contingent branching aligns the outcome distribution with
preferences), and the ambiguity is lower (the sharper observation
resolves more uncertainty about the lane).

\subsection{Belief Update and Second-Step Policy Selection}\label{app:step2}

After repositioning, the player observes $y = c$ (a clear lane).
Bayes' rule updates the belief about the lane state:
\begin{align}
    q(x{=}O \,|\, y{=}c)
    &= \frac{p(O)\,p(c \,|\, O,\, u_{\mathrm{rep}})}
            {p(O)\,p(c \,|\, O,\, u_{\mathrm{rep}})
             + p(B)\,p(c \,|\, B,\, u_{\mathrm{rep}})} \notag\\
    &= \frac{0.6 \times 0.9}{0.6 \times 0.9 + 0.4 \times 0.2}
    = \frac{0.54}{0.62}
    \approx 0.871\,.
\end{align}
The repositioning action has substantially sharpened the belief from
$(0.6,\, 0.4)$ to $(0.871,\, 0.129)$.

The agent now selects $u_2 \in \{u_{\mathrm{pass}},\,
u_{\mathrm{rec}}\}$ by comparing the risk component of the EFE under
the updated belief $q(x | y{=}c)$. (For simplicity we omit the
ambiguity term, which does not affect the ranking in this example.)

The predicted outcome distributions are
\begin{align}
    q(x'{=}A \,|\, u_{\mathrm{pass}})
    &= 0.871 \cdot 0.9 + 0.129 \cdot 0.2 = 0.810\,,\notag\\
    q(x'{=}A \,|\, u_{\mathrm{rec}})
    &= 0.500\,,
\end{align}
and the corresponding risk values are
\begin{align}
    \mathrm{KL}\!\big(q(x'|u_{\mathrm{pass}})\,\big\|\,\hat{p}(x')\big) &\approx 0.037\,,\notag\\
    \mathrm{KL}\!\big(q(x'|u_{\mathrm{rec}})\,\big\|\,\hat{p}(x')\big) &\approx 0.511\,.
\end{align}
Since $G(u_{\mathrm{pass}}) < G(u_{\mathrm{rec}})$, the agent selects
$u_2 = u_{\mathrm{pass}}$: pass to $P_2$. The complete behavior
selected by the model is therefore
\begin{equation}
    \text{reposition} \;\rightarrow\; \text{observe clear lane}
    \;\rightarrow\; \text{pass}\,.
\end{equation}
Repositioning was selected at step~1 because it reduced both risk
(via contingent branching) and ambiguity (via a sharper observation).
After the clear observation shifted the belief to $q(x{=}O) = 0.871$,
the risk at step~2 decisively favored passing over recycling. This
illustrates how EFE minimization produces a tactically intelligible
two-step behavior pattern from a simple generative model.
