# Supplementary material for: Active Inference for Physical AI Agents -- An Engineering Perspective
Source: arXiv:2603.20927 source file (2026-03-21)
Supplement: Supplementary file 2 [file appendix-thermostat.tex]

\section{Thermostat Example: Detailed Derivations}\label{app:thermostat-vfe}

\subsection{Derivation of the Individual VFE}\label{app:thermostat-vfe-deriv}

Agent $A$ maintains a Gaussian variational distribution $q_A(x_A)=\mathcal{N}(x_A | \mu_A,v_A)$
over the true temperature $x_A$, with prior $p(x_A)=\mathcal{N}(x_A | \hat{x},\sigma_x^2)$ and
likelihood $p(y_A|x_A)=\mathcal{N}(y_A | x_A,\sigma_y^2)$.  Starting from the VFE definition:
\begin{align}
    F_A(\mu_A, v_A)
    &= \mathbb{E}_{q_A}\left[\log\frac{q_A(x_A)}{p(x_A,\,y_A)}\right] \notag \\
    &= \mathbb{E}_{q_A}[\log q_A(x_A)]
       - \mathbb{E}_{q_A}[\log p(y_A|x_A)]
       - \mathbb{E}_{q_A}[\log p(x_A)] \notag \\
    &= -\tfrac{1}{2}\ln(2\pi e\,v_A)
       + \tfrac{1}{2}\ln(2\pi\sigma_y^2) + \frac{(y_A-\mu_A)^2+v_A}{2\sigma_y^2}
       + \tfrac{1}{2}\ln(2\pi\sigma_x^2) + \frac{(\mu_A-\hat{x})^2+v_A}{2\sigma_x^2} \notag \\
    &= \frac{(\mu_A - \hat{x})^2 + v_A}{2\sigma_x^2}
     + \frac{(y_A - \mu_A)^2 + v_A}{2\sigma_y^2} \notag \\
    &\qquad - \tfrac{1}{2}\ln v_A + \mathrm{const.}
\end{align}
where we used $\mathbb{E}_{q_A}[(x_A-c)^2]=(\mu_A-c)^2+v_A$ for any constant~$c$, which follows
from $\mathbb{E}_{q_A}[x_A^2]=\mu_A^2+v_A$.  All terms independent of $(\mu_A,v_A)$ are absorbed
into the constant.

\subsection{Derivation of the Kalman Update}\label{app:thermostat-kalman}

Setting $\partial F_A/\partial\mu_A = 0$:
\begin{align}
    \frac{\partial F_A}{\partial \mu_A}
    &= \frac{\mu_A - \hat{x}}{\sigma_x^2} + \frac{\mu_A - y_A}{\sigma_y^2} = 0 \notag \\
    &\Longrightarrow\quad
    \mu_A^*\left(\frac{1}{\sigma_x^2}+\frac{1}{\sigma_y^2}\right)
    = \frac{\hat{x}}{\sigma_x^2}+\frac{y_A}{\sigma_y^2} \notag \\
    &\Longrightarrow\quad
    \mu_A^* = \frac{\hat{x}/\sigma_x^2 + y_A/\sigma_y^2}{1/\sigma_x^2 + 1/\sigma_y^2}\,.
\end{align}

Setting $\partial F_A/\partial v_A = 0$:
\begin{align}
    \frac{\partial F_A}{\partial v_A}
    &= \frac{1}{2\sigma_x^2} + \frac{1}{2\sigma_y^2} - \frac{1}{2v_A} = 0 \notag \\
    &\Longrightarrow\quad
    \frac{1}{v_A^*} = \frac{1}{\sigma_x^2}+\frac{1}{\sigma_y^2} \,.
\end{align}
Both are global minima: $F_A$ is strictly convex in $(\mu_A,v_A)$ since all second
derivatives are positive.

\subsection{Derivation of the Collective VFE}\label{app:thermostat-collective-vfe}

The joint generative model factors as
$p(y_A, y_B, x_A, x_B) = p(y_A|x_A)\,p(y_B|x_B)\,p(x_B|x_A)\,p(x_A)$,
with individual likelihoods $p(y_i|x_i)=\mathcal{N}(y_i | x_i,\sigma_y^2)$,
prior $p(x_A)=\mathcal{N}(x_A | \hat{x},\sigma_x^2)$, and coupling
$p(x_B|x_A)=\mathcal{N}(x_B | x_A+\delta,\sigma_c^2)$.
Under the mean-field approximation $q_C(x_A,x_B)=q_A(x_A)\,q_B(x_B)$
with $q_i=\mathcal{N}(x_i | \mu_i,v_i)$, the collective VFE is
\begin{align}
    F_C &= \mathbb{E}_{q_C}\left[\log\frac{q_C(x_A,x_B)}{p(y_A,y_B,x_A,x_B)}\right] \notag \\
    &= \mathbb{E}_{q_A}[\log q_A] - \mathbb{E}_{q_A}[\log p(y_A|x_A)] - \mathbb{E}_{q_A}[\log p(x_A)] \notag \\
    &\quad + \mathbb{E}_{q_B}[\log q_B] - \mathbb{E}_{q_B}[\log p(y_B|x_B)]
       - \mathbb{E}_{q_C}[\log p(x_B|x_A)]\,. \label{eq:fc-expand}
\end{align}
The first three terms are exactly $F_A(\mu_A,v_A)$
(see Appendix~\ref{app:thermostat-vfe}).
The last three terms give $F_{B|A}$.
The first two of these are agent $B$'s likelihood and entropy contributions:
\begin{equation}
    \mathbb{E}_{q_B}[\log q_B] - \mathbb{E}_{q_B}[\log p(y_B|x_B)]
    = \frac{(y_B-\mu_B)^2+v_B}{2\sigma_y^2} - \tfrac{1}{2}\ln v_B + \mathrm{const.}
\end{equation}

For the last term, $p(x_B|x_A)=\mathcal{N}(x_B | x_A+\delta,\sigma_c^2)$, so
\begin{equation}
    -\mathbb{E}_{q_C}[\log p(x_B|x_A)]
    = \tfrac{1}{2}\ln(2\pi\sigma_c^2)
    + \frac{\mathbb{E}_{q_C}[(x_B - x_A - \delta)^2]}{2\sigma_c^2}\,.
\end{equation}
Since $x_A$ and $x_B$ are independent under $q_C$,
\begin{align}
    \mathbb{E}_{q_C}[(x_B - x_A - \delta)^2]
    &= \mathbb{E}_{q_C}\bigl[((x_B-\mu_B) - (x_A-\mu_A) + (\mu_B-\mu_A-\delta))^2\bigr]
    \notag \\
    &= \underbrace{\mathbb{E}_{q_B}[(x_B-\mu_B)^2]}_{v_B}
     + \underbrace{\mathbb{E}_{q_A}[(x_A-\mu_A)^2]}_{v_A}
     + (\mu_B-\mu_A-\delta)^2\,,
\end{align}
where the cross-terms vanish by independence.
Substituting back:
\begin{equation}
    -\mathbb{E}_{q_C}[\log p(x_B|x_A)]
    = \frac{(\mu_B-\mu_A-\delta)^2 + v_A + v_B}{2\sigma_c^2} + \mathrm{const.}
\end{equation}
Adding the coupling term to agent $B$'s likelihood and entropy contributions gives $F_{B|A}$.
Assembling all terms in~\eqref{eq:fc-expand} then gives $F_C = F_A + F_{B|A}$.

\subsection{Derivation of the Coupled Updates and Posterior Variances}\label{app:thermostat-coupled-update}

Substituting the individual and conditional VFE expressions into $F_C = F_A + F_{B|A}$, the full collective VFE (keeping only terms that depend on $\mu_A$, $\mu_B$, $v_A$, or $v_B$) is
\begin{align}
    F_C &= \frac{(\mu_A-\hat{x})^2+v_A}{2\sigma_x^2}
          + \frac{(y_A-\mu_A)^2+v_A}{2\sigma_y^2}
          + \frac{(y_B-\mu_B)^2+v_B}{2\sigma_y^2} \notag\\
        &\quad + \frac{(\mu_B-\mu_A-\delta)^2+v_A+v_B}{2\sigma_c^2}
          - \tfrac{1}{2}\ln v_A - \tfrac{1}{2}\ln v_B
          + \mathrm{const.}\label{eq:fc-combined}
\end{align}

\textit{Optimal means.}
Setting $\partial F_C/\partial\mu_A = 0$:
\begin{align}
    \frac{\partial F_C}{\partial\mu_A}
    &= \frac{\mu_A - \hat{x}}{\sigma_x^2}
       + \frac{\mu_A - y_A}{\sigma_y^2}
       - \frac{\mu_B - \mu_A - \delta}{\sigma_c^2} = 0 \notag\\
    &\Longrightarrow\quad
    \mu_A\left(\frac{1}{\sigma_x^2}+\frac{1}{\sigma_y^2}+\frac{1}{\sigma_c^2}\right)
    = \frac{\hat{x}}{\sigma_x^2} + \frac{y_A}{\sigma_y^2} + \frac{\mu_B-\delta}{\sigma_c^2} \notag\\
    &\Longrightarrow\quad
    \mu_A = \frac{\hat{x}/\sigma_x^2 + y_A/\sigma_y^2 + (\mu_B-\delta)/\sigma_c^2}%
                 {1/\sigma_x^2 + 1/\sigma_y^2 + 1/\sigma_c^2}\,,
\end{align}
Setting $\partial F_C/\partial\mu_B = 0$:
\begin{align}
    \frac{\partial F_C}{\partial\mu_B}
    &= \frac{\mu_B - y_B}{\sigma_y^2}
       + \frac{\mu_B - \mu_A - \delta}{\sigma_c^2} = 0 \notag\\
    &\Longrightarrow\quad
    \mu_B\left(\frac{1}{\sigma_y^2}+\frac{1}{\sigma_c^2}\right)
    = \frac{y_B}{\sigma_y^2} + \frac{\mu_A+\delta}{\sigma_c^2} \notag\\
    &\Longrightarrow\quad
    \mu_B = \frac{y_B/\sigma_y^2 + (\mu_A+\delta)/\sigma_c^2}{1/\sigma_y^2 + 1/\sigma_c^2}\,,
\end{align}
Since $F_C$ is strictly convex in $(\mu_A,\mu_B)$, the pair of linear equations above has a unique solution, obtainable in closed form by back-substitution.

\textit{Optimal variances.}
The terms in \eqref{eq:fc-combined} that depend on $v_A$ are
\begin{equation}
    \frac{v_A}{2\sigma_x^2} + \frac{v_A}{2\sigma_y^2} + \frac{v_A}{2\sigma_c^2} - \tfrac{1}{2}\ln v_A\,.
\end{equation}
The third contribution ($v_A/2\sigma_c^2$) comes from the coupling term $(\mu_B-\mu_A-\delta)^2+v_A+v_B$: agent $A$'s own uncertainty propagates into agent $B$'s coupling cost, so minimizing $F_C$ over $v_A$ must account for this extra cost.  Setting $\partial F_C/\partial v_A = 0$:
\begin{equation}
    \frac{1}{2\sigma_x^2} + \frac{1}{2\sigma_y^2} + \frac{1}{2\sigma_c^2} - \frac{1}{2v_A} = 0
    \;\Longrightarrow\;
    \frac{1}{v_A^*} = \frac{1}{\sigma_x^2} + \frac{1}{\sigma_y^2} + \frac{1}{\sigma_c^2}\,.
    \label{eq:va-coupled-result}
\end{equation}

The terms in \eqref{eq:fc-combined} that depend on $v_B$ are
\begin{equation}
    \frac{v_B}{2\sigma_y^2} + \frac{v_B}{2\sigma_c^2} - \tfrac{1}{2}\ln v_B\,.
\end{equation}
Agent $B$ has no independent prior (the wall coupling serves as its prior), so only the observation and coupling precisions contribute.  Setting $\partial F_C/\partial v_B = 0$:
\begin{equation}
    \frac{1}{2\sigma_y^2} + \frac{1}{2\sigma_c^2} - \frac{1}{2v_B} = 0
    \;\Longrightarrow\;
    \frac{1}{v_B^*} = \frac{1}{\sigma_y^2} + \frac{1}{\sigma_c^2}\,.
    \label{eq:vb-coupled-result}
\end{equation}

The asymmetry $v_A^* < v_B^*$ reflects the structure of the joint model: the coupling $p(x_B|x_A)$ acts as a \emph{conditional prior} for~$B$ (contributing $\sigma_c^{-2}$ to $B$'s precision) but also as an extra cost on~$A$ (since $A$'s variance $v_A$ appears inside the coupling term).  Agent~$A$ therefore benefits from three precision sources, agent~$B$ from only two.  With $\sigma_x^2=4$, $\sigma_y^2=1$, $\sigma_c^2=1$:
\begin{equation}
    v_A^* = (0.25+1+1)^{-1} = 0.44\,^\circ\mathrm{C}^2\,,\qquad
    v_B^* = (1+1)^{-1} = 0.50\,^\circ\mathrm{C}^2\,,
\end{equation}
confirming the numerical values stated in the main text.

\subsection{Derivation of the Three-Term VFE}\label{app:vfe-three-terms}

\textit{Recognition model.}
The collective transition
\begin{equation}\label{eq:collective-state-pred}
    q(x'|u) = \mathcal{N}(x' | u,\, \sigma_u^2/N)\,,
\end{equation}
inverted under a flat prior on $u$, yields the recognition model:
\begin{equation}\label{eq:recognition-model}
    q(u|x') = \mathcal{N}(u | x',\, \sigma_u^2/N)\,.
\end{equation}

\textit{Joint generative model.}
The rollout $(x',y',u)$ is governed by:
\begin{equation}\label{eq:planning-joint}
    p(x',y',u) = \hat{p}(x')\,p(y'|x')\,q(u|x')\,,
\end{equation}
with
\begin{align*}
    \hat{p}(x') &= \mathcal{N}(x' | x^*,\sigma_\mathrm{goal}^2)\,, \\
    p(y'|x') &= \mathcal{N}(y' | x',\sigma_y^2/N)\,.
\end{align*}

\textit{Variational distribution.}
For fixed policy $u$, the agent's joint over $(x',y')$ is:
\begin{equation}\label{eq:planning-variational}
    q(x',y'|u) = q(x'|u)\,p(y'|x')\,.
\end{equation}

\textit{VFE expansion.}
Computing the KL divergence $\mathbb{E}_{q(x',y'|u)}[\log q(x',y'|u) - \log p(x',y',u)]$ and noting that $\log p(y'|x')$ appears with opposite signs in $\log q$ and $\log p$ and therefore cancels:
\begin{align}
    F_N(u)
    &= \mathbb{E}_{q(x'|u)}\bigl[\log q(x'|u) - \log \hat{p}(x')\bigr]
       - \mathbb{E}_{q(x'|u)}\bigl[\log q(u|x')\bigr] \notag\\
    &= \mathrm{KL}\bigl[q(x'|u)\,\big\|\,\hat{p}(x')\bigr]
       + \mathbb{H}\bigl[q(u|x')\bigr]\,. \label{eq:vfe-two-terms-N}
\end{align}

\textit{Three-term grouping.}
Adding and subtracting the ambiguity $\mathbb{H}[p(y'|x')]$:
\begin{align}\label{eq:cross-term-N}
    F_N(u)
    &= \underbrace{\mathrm{KL}\bigl[q(x'|u)\,\big\|\,\hat{p}(x')\bigr]}_{\text{risk}}
       + \underbrace{\mathbb{H}\bigl[p(y'|x')\bigr]}_{\text{ambiguity}}
       + \underbrace{\mathbb{H}\bigl[q(u|x')\bigr] - \mathbb{H}\bigl[p(y'|x')\bigr]}_{\text{cross-term}}\,.
\end{align}
Using $\mathbb{H}[q(u|x')] - \mathbb{H}[p(y'|x')] = \mathbb{E}_q\bigl[\log p(y'|x') - \log q(u|x')\bigr]$ gives the three-term VFE decomposition.
For the Gaussian models \eqref{eq:collective-state-pred}--\eqref{eq:recognition-model}, the entropies are $\mathbb{H}[q(u|x')] = \tfrac{1}{2}\log(2\pi e\,\sigma_u^2/N)$ and $\mathbb{H}[p(y'|x')] = \tfrac{1}{2}\log(2\pi e\,\sigma_y^2/N)$, giving the constant cross-term $\tfrac{1}{2}\log(\sigma_u^2/\sigma_y^2)$ reported in \eqref{eq:cross-term-N}.
