# Supplementary material for: Active Inference for Physical AI Agents -- An Engineering Perspective
Source: arXiv:2603.20927 source file (2026-03-21)
Supplement: Supplementary file 3 [file appendix.tex]

\appendix
\section{Proofs}

\subsection{Proof of the complexity-accuracy decomposition}
\begin{subequations}\label{eq:proof-surprise}
    \begin{align}
    \underbrace{ -\log p(D|m)}_{\text{surprisal}} &=  -\log p(D|m) \underbrace{\int p(\theta|D,m)\mathrm{d}\theta}_{=1}  \\
     &= \int p(\theta|D,m)\log \frac{1}{p(D|m)}\mathrm{d}\theta \\
     &= \int p(\theta|D,m)\log \underbrace{\frac{p(\theta|D,m)}{p(D|\theta,m) p(\theta|m)}}_{\text{by Bayes rule}}\mathrm{d}\theta \\
     &= \underbrace{\int p(\theta|D,m)\log \frac{p(\theta|D,m)}{ p(\theta|m)}\mathrm{d}\theta}_{\text{complexity}} - \underbrace{\int p(\theta|D,m)\log p(D|\theta,m)\mathrm{d}\theta}_{\text{accuracy ("data fit")}}
\end{align}
\end{subequations}

\subsection{Proof of Equation~\ref{eq:auto-states-dynamics}}

We derive Eq.~\eqref{eq:auto-states-dynamics}, showing that the autonomous states of an agent evolve along the gradient of the log steady-state density, starting from assumptions F1--F3.  This derivation follows the arguments laid out by Friston in \cite[Part~One, Sections~1--2]{fristonfree2019} and \cite[Section~2]{fristonlife2013}, with further discussion in \cite{parrmarkov2020} and \cite{kirchhoffmarkov2018}.

%---------------------------------------------------------------------
\subsection*{Step 1: Fokker--Planck Equation from the Langevin Dynamics (F1)}

Assumption F1 states that the combined system--environment states evolve according to a Langevin equation \cite[Eq.~(1.1)]{fristonfree2019}:
\begin{equation}\label{eq:langevin}
    \dot{z} = f(z) + \omega, \qquad \omega \sim \mathcal{N}(0,\, 2\Gamma),
\end{equation}
where $z$ collects all states, $f(z)$ is the deterministic flow, and $\Gamma$ is a symmetric positive-semidefinite diffusion matrix.

By standard results in stochastic calculus, the time evolution of the probability density $p(z,t)$ over states is governed by the Fokker--Planck equation \cite[Eq.~(1.6)]{fristonfree2019}:
\begin{equation}\label{eq:FP}
    \frac{\partial p(z,t)}{\partial t}
    = -\nabla \cdot \bigl[\, f(z)\, p(z,t) \,\bigr]
      + \nabla \cdot \bigl[\, \Gamma\, \nabla p(z,t) \,\bigr].
\end{equation}
This can be written as a continuity equation,
\begin{equation}
    \frac{\partial p}{\partial t} = -\nabla \cdot j(z,t),
\end{equation}
with probability current
\begin{equation}\label{eq:current}
    j(z,t) = f(z)\, p(z,t) - \Gamma\, \nabla p(z,t).
\end{equation}

%---------------------------------------------------------------------
\subsection*{Step 2: Helmholtz Decomposition at Steady State (F2)}

Assumption F2 states that the system admits a non-equilibrium steady-state (NESS) density $p(z)$, so that
\begin{equation}
    \frac{\partial p}{\partial t} = 0
    \qquad \Longrightarrow \qquad
    \nabla \cdot j = 0.
\end{equation}

At steady state, the flow $f(z)$ can be decomposed via a \textbf{Helmholtz decomposition} into dissipative and solenoidal components \cite[Eq.~(1.7)]{fristonfree2019}, \cite{aopotential2004}.  Using the relation $\Im(z) = -\log p(z)$ for the surprisal (or self-information), the flow takes the form \cite[Eq.~(1.8)]{fristonfree2019}:
\begin{equation}\label{eq:helmholtz}
    \boxed{f(z) = \bigl(\Gamma + Q(z)\bigr)\, \nabla \log p(z),}
\end{equation}
where $\Gamma = \Gamma^\top \succeq 0$ is the (symmetric) diffusion matrix and $Q(z) = -Q(z)^\top$ is an antisymmetric matrix encoding solenoidal (divergence-free) flow.

\subsubsection{Verification} Substituting \eqref{eq:helmholtz} into the probability current \eqref{eq:current}:
\begin{align}
    j &= f\, p - \Gamma\, \nabla p \notag\\
      &= \bigl(\Gamma + Q\bigr)(\nabla \log p)\, p - \Gamma\, \nabla p \notag\\
      &= \bigl(\Gamma + Q\bigr)\, \nabla p - \Gamma\, \nabla p \notag\\
      &= Q\, \nabla p, \label{eq:solenoid_current}
\end{align}
where we used $(\nabla \log p)\, p = \nabla p$.  Since $Q$ is antisymmetric, $\nabla \cdot (Q\, \nabla p) = 0$ under suitable regularity conditions, confirming $\nabla \cdot j = 0$.  This is precisely the result established in \cite[Eq.~(1.8), second line]{fristonfree2019} and discussed in \cite[Section~2(a)]{fristonfree2019}.

The two components have distinct roles:
\begin{itemize}[itemsep=4pt]
    \item \textbf{Dissipative (gradient) flow:} $\Gamma\, \nabla \log p(z)$, which drives the system toward regions of higher $p(z)$.
    \item \textbf{Solenoidal (curl) flow:} $Q(z)\, \nabla \log p(z)$, which circulates probability without changing the density.
\end{itemize}

%---------------------------------------------------------------------
\subsection*{Step 3: Markov Blanket Partition (F3)}

Assumption F3 partitions the states as $z = (y,\, x,\, u,\, s)$, where:
\begin{center}
\begin{tabular}{cl}
    $y$ & sensory states, \\
    $x$ & external (environmental) states, \\
    $u$ & control (active) states, \\
    $s$ & internal (agent) states.
\end{tabular}
\end{center}
The sensory and control states $(y, u)$ form a \textbf{Markov blanket}, enforcing the conditional independence \cite[Section~1.4]{fristonfree2019}, \cite[Fig.~1]{fristonlife2013}, \cite{kirchhoffmarkov2018}:
\begin{equation}\label{eq:markov}
    x \perp s | (y,\, u).
\end{equation}

Define the \textbf{autonomous states} $\alpha \triangleq (u,\, s)$.  By the Markov blanket condition, the dynamics of $\alpha$ are not directly driven by external states.  This follows from the sparse coupling structure implied by the Markov blanket: the flow of autonomous states, and the corresponding blocks of the diffusion and solenoidal matrices, depend only on blanket and internal states \cite[Section~1.5, Marginal Flow Lemma]{fristonfree2019}:
\begin{equation}\label{eq:decouple}
    f_\alpha(z) = f_\alpha(y,\, u,\, s),
    \qquad
    \Gamma_{\alpha\alpha} = \Gamma_{\alpha\alpha}(y,\, u,\, s),
    \qquad
    Q_{\alpha\alpha} = Q_{\alpha\alpha}(y,\, u,\, s).
\end{equation}

%---------------------------------------------------------------------
\subsection*{Step 4: Projecting the Helmholtz Decomposition onto Autonomous States}

Restricting the Helmholtz decomposition \eqref{eq:helmholtz} to the autonomous states $\alpha = (u,s)$ gives the $\alpha$-components of the flow.  This step invokes the \emph{marginal flow lemma} of \cite[Eq.~(1.22)]{fristonfree2019}, which shows that the marginal flow of any subset of states can be expressed in terms of the NESS density and the corresponding sub-blocks of $\Gamma$ and $Q$:
\begin{equation}\label{eq:restricted}
    f_\alpha = \bigl(\Gamma_{\alpha\alpha} + Q_{\alpha\alpha}\bigr)\, \nabla_\alpha \log p(z).
\end{equation}

Now, the Markov blanket factorization of the NESS density gives (as a consequence of \eqref{eq:markov}):
\begin{equation}\label{eq:factor}
    p(z) = p(y,\, x,\, u,\, s) = p(x | y,\, u)\; p(y,\, u,\, s).
\end{equation}
Taking the gradient with respect to $\alpha = (u,s)$:
\begin{equation}\label{eq:grad_split}
    \nabla_\alpha \log p(z)
    = \underbrace{\nabla_\alpha \log p(x | y,\, u)}_{\text{(i)}}
    + \underbrace{\nabla_\alpha \log p(y,\, u,\, s)}_{\text{(ii)}}.
\end{equation}

\subsubsection{Eliminating term (i)}
By the Markov blanket condition \eqref{eq:markov}, $p(x | y, u)$ does not depend on the internal states $s$, so
\begin{equation}
    \nabla_s \log p(x | y,\, u) = 0.
\end{equation}
The remaining contribution $\nabla_u \log p(x | y, u)$, when pre-multiplied by $(\Gamma_{\alpha\alpha} + Q_{\alpha\alpha})$, contributes only to the solenoidal (non-dissipative) component of the flow.  In Friston's treatment \cite[Section~8, Eq.~(8.5) and surrounding discussion]{fristonfree2019}, \cite[Section~2(b)]{fristonlife2013}, this term is absorbed into the solenoidal flow $Q_{\alpha\alpha}$ and does not contribute to the gradient (dissipative) dynamics.  

\subsubsection{Result}  Retaining the dominant gradient flow, the dynamics of the autonomous states are therefore:

\begin{equation}\label{eq:result}
    \boxed{\dot{\alpha} \propto \nabla_\alpha \log p(y,\, u,\, s).}
\end{equation}

The proportionality conceals the matrix prefactor $(\Gamma_{\alpha\alpha} + Q_{\alpha\alpha})$:
\begin{itemize}[itemsep=4pt]
    \item $\Gamma_{\alpha\alpha}\, \nabla_\alpha \log p(y,u,s)$ is the \textbf{dissipative} component, performing gradient ascent on the log-density and driving the agent toward high-probability regions.
    \item $Q_{\alpha\alpha}\, \nabla_\alpha \log p(y,u,s)$ is the \textbf{solenoidal} component, which rotates the flow without changing $-\log p$.
\end{itemize}

\subsection*{Interpretation}

Equation \eqref{eq:result} states that the agent's internal and active states evolve so as to ascend the log steady-state density $\log p(y,u,s)$.  Equivalently, they perform gradient \emph{descent} on the surprisal (self-information) \cite[Section~1.2]{fristonfree2019}:
\begin{equation}
    \dot{\alpha} \propto -\nabla_\alpha \bigl[-\log p(y,\, u,\, s)\bigr].
\end{equation}
Whenever the system drifts toward regions of lower steady-state probability, the dynamics push it back toward more probable configurations, thereby maintaining the agent's recognizable form.  This is the core mathematical content of the Free Energy Principle \cite{fristonfree2019,fristonlife2013}.

\subsubsection{Remark on technical caveats}

Biehl et al.\ \cite{biehltechnical2021} have raised technical concerns about the generality of several steps in this derivation, particularly regarding the rewriting of the equations of motion under the Markov blanket partition and the conditions under which the free energy lemma holds.  Friston et al.\ \cite{fristoninteresting2021} responded by clarifying the role of solenoidal coupling and the distinction between exact and approximate Bayesian inference.  The reader is referred to these works for a discussion of the precise mathematical conditions required.




\subsection{Thermostat Example: Detailed Derivations}\label{app:thermostat-vfe}

\subsubsection{Derivation of VFE~\eqref{eq:thermostat-vfe-a}}

Agent $A$ maintains a Gaussian variational distribution $q_A(x_A)=\mathcal{N}(x_A | \mu_A,v_A)$
over the true temperature $x_A$, with prior $p(x_A)=\mathcal{N}(x_A | \hat{x},\sigma_x^2)$ and
likelihood $p(y_A|x_A)=\mathcal{N}(y_A | x_A,\sigma_y^2)$.  Starting from the VFE definition:
\begin{align}
    F_A(\mu_A, v_A)
    &= \mathbb{E}_{q_A}\left[\log\frac{q_A(x_A)}{p(x_A,\,y_A)}\right] \notag \\
    &= \mathbb{E}_{q_A}[\log q_A(x_A)]
       - \mathbb{E}_{q_A}[\log p(y_A|x_A)]
       - \mathbb{E}_{q_A}[\log p(x_A)] \notag \\
    &= -\tfrac{1}{2}\ln(2\pi e\,v_A)
       + \tfrac{1}{2}\ln(2\pi\sigma_y^2) + \frac{(y_A-\mu_A)^2+v_A}{2\sigma_y^2}
       + \tfrac{1}{2}\ln(2\pi\sigma_x^2) + \frac{(\mu_A-\hat{x})^2+v_A}{2\sigma_x^2} \notag \\
    &= \frac{(\mu_A - \hat{x})^2 + v_A}{2\sigma_x^2}
     + \frac{(y_A - \mu_A)^2 + v_A}{2\sigma_y^2}
     - \tfrac{1}{2}\ln v_A + \mathrm{const.}
\end{align}
where we used $\mathbb{E}_{q_A}[(x_A-c)^2]=(\mu_A-c)^2+v_A$ for any constant~$c$, which follows
from $\mathbb{E}_{q_A}[x_A^2]=\mu_A^2+v_A$.  All terms independent of $(\mu_A,v_A)$ are absorbed
into the constant.

\subsubsection{Derivation of the Kalman Update~\eqref{eq:thermostat-solo}}\label{app:thermostat-kalman}

Setting $\partial F_A/\partial\mu_A = 0$:
\begin{align}
    \frac{\partial F_A}{\partial \mu_A}
    &= \frac{\mu_A - \hat{x}}{\sigma_x^2} + \frac{\mu_A - y_A}{\sigma_y^2} = 0 \notag \\
    &\Longrightarrow\quad
    \mu_A^*\left(\frac{1}{\sigma_x^2}+\frac{1}{\sigma_y^2}\right)
    = \frac{\hat{x}}{\sigma_x^2}+\frac{y_A}{\sigma_y^2} \notag \\
    &\Longrightarrow\quad
    \mu_A^* = \frac{\hat{x}/\sigma_x^2 + y_A/\sigma_y^2}{1/\sigma_x^2 + 1/\sigma_y^2}\,.
\end{align}

Setting $\partial F_A/\partial v_A = 0$:
\begin{align}
    \frac{\partial F_A}{\partial v_A}
    &= \frac{1}{2\sigma_x^2} + \frac{1}{2\sigma_y^2} - \frac{1}{2v_A} = 0 \notag \\
    &\Longrightarrow\quad
    \frac{1}{v_A^*} = \frac{1}{\sigma_x^2}+\frac{1}{\sigma_y^2} \,.
\end{align}
Both are global minima: $F_A$ is strictly convex in $(\mu_A,v_A)$ since all second
derivatives are positive.

\subsubsection{Derivation of the Collective VFE~\eqref{eq:thermostat-collective-vfe}}\label{app:thermostat-collective-vfe}

The joint generative model factors as
$p(y_A, y_B, x_A, x_B) = p(y_A|x_A)\,p(y_B|x_B)\,p(x_B|x_A)\,p(x_A)$,
with individual likelihoods $p(y_i|x_i)=\mathcal{N}(y_i | x_i,\sigma_y^2)$,
prior $p(x_A)=\mathcal{N}(x_A | \hat{x},\sigma_x^2)$, and coupling
$p(x_B|x_A)=\mathcal{N}(x_B | x_A+\delta,\sigma_c^2)$.
Under the mean-field approximation $q_C(x_A,x_B)=q_A(x_A)\,q_B(x_B)$
with $q_i=\mathcal{N}(x_i | \mu_i,v_i)$, the collective VFE is
\begin{align}
    F_C &= \mathbb{E}_{q_C}\left[\log\frac{q_C(x_A,x_B)}{p(y_A,y_B,x_A,x_B)}\right] \notag \\
    &= \mathbb{E}_{q_A}[\log q_A] - \mathbb{E}_{q_A}[\log p(y_A|x_A)] - \mathbb{E}_{q_A}[\log p(x_A)] \notag \\
    &\quad + \mathbb{E}_{q_B}[\log q_B] - \mathbb{E}_{q_B}[\log p(y_B|x_B)]
       - \mathbb{E}_{q_C}[\log p(x_B|x_A)]\,. \label{eq:fc-expand}
\end{align}
The first three terms are exactly $F_A(\mu_A,v_A)$
(see Appendix~\ref{app:thermostat-vfe}).
The last three terms give $F_{B|A}$~\eqref{eq:thermostat-vfe-bca}.
The first two of these are agent $B$'s likelihood and entropy contributions:
\begin{equation}
    \mathbb{E}_{q_B}[\log q_B] - \mathbb{E}_{q_B}[\log p(y_B|x_B)]
    = \frac{(y_B-\mu_B)^2+v_B}{2\sigma_y^2} - \tfrac{1}{2}\ln v_B + \mathrm{const.}
\end{equation}

For the last term, $p(x_B|x_A)=\mathcal{N}(x_B | x_A+\delta,\sigma_c^2)$, so
\begin{equation}
    -\mathbb{E}_{q_C}[\log p(x_B|x_A)]
    = \tfrac{1}{2}\ln(2\pi\sigma_c^2)
    + \frac{\mathbb{E}_{q_C}[(x_B - x_A - \delta)^2]}{2\sigma_c^2}\,.
\end{equation}
Since $x_A$ and $x_B$ are independent under $q_C$,
\begin{align}
    \mathbb{E}_{q_C}[(x_B - x_A - \delta)^2]
    &= \mathbb{E}_{q_C}\bigl[((x_B-\mu_B) - (x_A-\mu_A) + (\mu_B-\mu_A-\delta))^2\bigr]
    \notag \\
    &= \underbrace{\mathbb{E}_{q_B}[(x_B-\mu_B)^2]}_{v_B}
     + \underbrace{\mathbb{E}_{q_A}[(x_A-\mu_A)^2]}_{v_A}
     + (\mu_B-\mu_A-\delta)^2\,,
\end{align}
where the cross-terms vanish by independence.
Substituting back:
\begin{equation}
    -\mathbb{E}_{q_C}[\log p(x_B|x_A)]
    = \frac{(\mu_B-\mu_A-\delta)^2 + v_A + v_B}{2\sigma_c^2} + \mathrm{const.}
\end{equation}
Adding the coupling term to agent $B$'s likelihood and entropy contributions gives $F_{B|A}$~\eqref{eq:thermostat-vfe-bca}.
Assembling all terms in~\eqref{eq:fc-expand} then gives $F_C = F_A + F_{B|A}$, i.e., \eqref{eq:thermostat-collective-vfe}.

\subsubsection{Derivation of the Coupled Updates~\eqref{eq:coupled-update-a}--\eqref{eq:coupled-update-b} and Posterior Variances}\label{app:thermostat-coupled-update}

Substituting \eqref{eq:thermostat-vfe-a} and \eqref{eq:thermostat-vfe-bca} into $F_C = F_A + F_{B|A}$, the full collective VFE (keeping only terms that depend on $\mu_A$, $\mu_B$, $v_A$, or $v_B$) is
\begin{align}
    F_C &= \frac{(\mu_A-\hat{x})^2+v_A}{2\sigma_x^2}
          + \frac{(y_A-\mu_A)^2+v_A}{2\sigma_y^2}
          + \frac{(y_B-\mu_B)^2+v_B}{2\sigma_y^2} \notag\\
        &\quad + \frac{(\mu_B-\mu_A-\delta)^2+v_A+v_B}{2\sigma_c^2}
          - \tfrac{1}{2}\ln v_A - \tfrac{1}{2}\ln v_B
          + \mathrm{const.}\label{eq:fc-combined}
\end{align}

\textit{Optimal means.}
Setting $\partial F_C/\partial\mu_A = 0$:
\begin{align}
    \frac{\partial F_C}{\partial\mu_A}
    &= \frac{\mu_A - \hat{x}}{\sigma_x^2}
       + \frac{\mu_A - y_A}{\sigma_y^2}
       - \frac{\mu_B - \mu_A - \delta}{\sigma_c^2} = 0 \notag\\
    &\Longrightarrow\quad
    \mu_A\left(\frac{1}{\sigma_x^2}+\frac{1}{\sigma_y^2}+\frac{1}{\sigma_c^2}\right)
    = \frac{\hat{x}}{\sigma_x^2} + \frac{y_A}{\sigma_y^2} + \frac{\mu_B-\delta}{\sigma_c^2} \notag\\
    &\Longrightarrow\quad
    \mu_A = \frac{\hat{x}/\sigma_x^2 + y_A/\sigma_y^2 + (\mu_B-\delta)/\sigma_c^2}%
                 {1/\sigma_x^2 + 1/\sigma_y^2 + 1/\sigma_c^2}\,,
\end{align}
which is \eqref{eq:coupled-update-a}.

Setting $\partial F_C/\partial\mu_B = 0$:
\begin{align}
    \frac{\partial F_C}{\partial\mu_B}
    &= \frac{\mu_B - y_B}{\sigma_y^2}
       + \frac{\mu_B - \mu_A - \delta}{\sigma_c^2} = 0 \notag\\
    &\Longrightarrow\quad
    \mu_B\left(\frac{1}{\sigma_y^2}+\frac{1}{\sigma_c^2}\right)
    = \frac{y_B}{\sigma_y^2} + \frac{\mu_A+\delta}{\sigma_c^2} \notag\\
    &\Longrightarrow\quad
    \mu_B = \frac{y_B/\sigma_y^2 + (\mu_A+\delta)/\sigma_c^2}{1/\sigma_y^2 + 1/\sigma_c^2}\,,
\end{align}
which is \eqref{eq:coupled-update-b}.  Since $F_C$ is strictly convex in $(\mu_A,\mu_B)$, the pair of linear equations~\eqref{eq:coupled-update-a}--\eqref{eq:coupled-update-b} has a unique solution, obtainable in closed form by substituting \eqref{eq:coupled-update-b} into \eqref{eq:coupled-update-a}.

\textit{Optimal variances.}
The terms in \eqref{eq:fc-combined} that depend on $v_A$ are
\begin{equation}
    \frac{v_A}{2\sigma_x^2} + \frac{v_A}{2\sigma_y^2} + \frac{v_A}{2\sigma_c^2} - \tfrac{1}{2}\ln v_A\,.
\end{equation}
The third contribution ($v_A/2\sigma_c^2$) comes from the coupling term $(\mu_B-\mu_A-\delta)^2+v_A+v_B$: agent $A$'s own uncertainty propagates into agent $B$'s coupling cost, so minimizing $F_C$ over $v_A$ must account for this extra cost.  Setting $\partial F_C/\partial v_A = 0$:
\begin{equation}
    \frac{1}{2\sigma_x^2} + \frac{1}{2\sigma_y^2} + \frac{1}{2\sigma_c^2} - \frac{1}{2v_A} = 0
    \;\Longrightarrow\;
    \frac{1}{v_A^*} = \frac{1}{\sigma_x^2} + \frac{1}{\sigma_y^2} + \frac{1}{\sigma_c^2}\,.
    \label{eq:va-coupled-result}
\end{equation}

The terms in \eqref{eq:fc-combined} that depend on $v_B$ are
\begin{equation}
    \frac{v_B}{2\sigma_y^2} + \frac{v_B}{2\sigma_c^2} - \tfrac{1}{2}\ln v_B\,.
\end{equation}
Agent $B$ has no independent prior (the wall coupling serves as its prior), so only the observation and coupling precisions contribute.  Setting $\partial F_C/\partial v_B = 0$:
\begin{equation}
    \frac{1}{2\sigma_y^2} + \frac{1}{2\sigma_c^2} - \frac{1}{2v_B} = 0
    \;\Longrightarrow\;
    \frac{1}{v_B^*} = \frac{1}{\sigma_y^2} + \frac{1}{\sigma_c^2}\,.
    \label{eq:vb-coupled-result}
\end{equation}

The asymmetry $v_A^* < v_B^*$ reflects the structure of the joint model: the coupling $p(x_B|x_A)$ acts as a \emph{conditional prior} for~$B$ (contributing $\sigma_c^{-2}$ to $B$'s precision) but also as an extra cost on~$A$ (since $A$'s variance $v_A$ appears inside the coupling term).  Agent~$A$ therefore benefits from three precision sources, agent~$B$ from only two.  With $\sigma_x^2=4$, $\sigma_y^2=1$, $\sigma_c^2=1$:
\begin{equation}
    v_A^* = (0.25+1+1)^{-1} = 0.44\,^\circ\mathrm{C}^2\,,\qquad
    v_B^* = (1+1)^{-1} = 0.50\,^\circ\mathrm{C}^2\,,
\end{equation}
confirming \eqref{eq:thermostat-coupled-nums}.

\subsubsection{Derivation of the Three-Term VFE~\eqref{eq:vfe-three-terms}}\label{app:vfe-three-terms}

\textit{Recognition model.}
The collective transition $q(x'|u) = \mathcal{N}(x' | u,\, \sigma_u^2/N)$, inverted under a flat prior on $u$, yields the recognition model:
\begin{equation}\label{eq:recognition-model}
    q(u|x') = \mathcal{N}(u | x',\, \sigma_u^2/N)\,.
\end{equation}

\textit{Joint generative model.}
The rollout $(x',y',u)$ is governed by:
\begin{equation}\label{eq:planning-joint}
    p(x',y',u) = \hat{p}(x')\,p(y'|x')\,q(u|x')\,,
\end{equation}
with preference prior $\hat{p}(x') = \mathcal{N}(x' | x^*,\sigma_\mathrm{goal}^2)$ and future observation model $p(y'|x') = \mathcal{N}(y' | x',\sigma_y^2/N)$.

\textit{Variational distribution.}
For fixed policy $u$, the agent's joint over $(x',y')$ is:
\begin{equation}\label{eq:planning-variational}
    q(x',y'|u) = q(x'|u)\,p(y'|x')\,.
\end{equation}

\textit{VFE expansion.}
Computing the KL divergence $\mathbb{E}_{q(x',y'|u)}[\log q(x',y'|u) - \log p(x',y',u)]$ and noting that $\log p(y'|x')$ appears with opposite signs in $\log q$ and $\log p$ and therefore cancels:
\begin{align}
    F_N(u)
    &= \mathbb{E}_{q(x'|u)}\bigl[\log q(x'|u) - \log \hat{p}(x')\bigr]
       - \mathbb{E}_{q(x'|u)}\bigl[\log q(u|x')\bigr] \notag\\
    &= \mathrm{KL}\bigl[q(x'|u)\,\big\|\,\hat{p}(x')\bigr]
       + \mathbb{H}\bigl[q(u|x')\bigr]\,. \label{eq:vfe-two-terms-N}
\end{align}

\textit{Three-term grouping.}
Adding and subtracting the ambiguity $\mathbb{H}[p(y'|x')]$:
\begin{align}
    F_N(u)
    &= \underbrace{\mathrm{KL}\bigl[q(x'|u)\,\big\|\,\hat{p}(x')\bigr]}_{\text{risk}}
       + \underbrace{\mathbb{H}\bigl[p(y'|x')\bigr]}_{\text{ambiguity}}
       + \underbrace{\mathbb{H}\bigl[q(u|x')\bigr] - \mathbb{H}\bigl[p(y'|x')\bigr]}_{\text{cross-term}}\,.
\end{align}
Using $\mathbb{H}[q(u|x')] - \mathbb{H}[p(y'|x')] = \mathbb{E}_q\bigl[\log p(y'|x') - \log q(u|x')\bigr]$ recovers \eqref{eq:vfe-three-terms}.
For the Gaussian models \eqref{eq:collective-state-pred}--\eqref{eq:recognition-model}, the entropies are $\mathbb{H}[q(u|x')] = \tfrac{1}{2}\log(2\pi e\,\sigma_u^2/N)$ and $\mathbb{H}[p(y'|x')] = \tfrac{1}{2}\log(2\pi e\,\sigma_y^2/N)$, giving the constant cross-term $\tfrac{1}{2}\log(\sigma_u^2/\sigma_y^2)$ reported in \eqref{eq:cross-term-N}.

\subsection*{Sample Bio}
\begin{IEEEbiographynophoto}{First Author Name}
(~\IEEEmembership{Member,~IEEE}) received his B.S. degree from the Insert College Name and his M.S. and Ph.D. degrees from University Name. He was a postdoctoral researcher at the Company Name and is now a job position at University/Company Name, University/Company City, State, Postal Code, Country. He is a recipient of the Insert Your Award Name Prize. His research focuses on the design, analysis, and implementation of algorithms for large-scale nonlinear optimization problems. He is a Member of IEEE.
\end{IEEEbiographynophoto}
%
\vspace{11pt} % To separate multiple biographies

\begin{IEEEbiographynophoto}{Second Author Name}
(~\IEEEmembership{Fellow,~IEEE}) received his B.S. degree from the Insert College Name and his M.S. and Ph.D. degrees from University Name. He was a postdoctoral researcher at the Company Name and is now a job position at University/Company Name, University/Company City, State, Postal Code, Country. He is a recipient of the Insert Your Award Name Prize. His research focuses on the design, analysis, and implementation of algorithms for large-scale nonlinear optimization problems. He is a Member of IEEE.
\end{IEEEbiographynophoto}

\vfill
